# Supplementary material for: Online estimation of the hand-eye transformation from surgical scenes
Source: arXiv:2306.02261 source file (2023-06-04)
Supplement: Supplementary file 1 [file suppplementary-formula.tex]

\documentclass[sn-mathphys]{sn-jnl}% Math and Physical Sciences Reference Style

\usepackage{graphics}
\usepackage{subfigure}
\usepackage{epsfig}
\usepackage{amsmath} 
\usepackage{amssymb}  

\begin{document}

\section*{Derivative of the objective functions}
Since the learning of any network is done through back-propagation and gradient descent, the objective function used in the network must be differentiable, i.e. the gradient with respect to learned parameters must exist. This section shows that the functions used in the paper have a valid gradient with respect to the network parameters $\vec{x} = [x_1, x_2, ..., x_N]^T$, where $N$ is the number of learnable parameters.
\subsection*{Constructing the hand-eye transformation}
The hand-eye transformation in the paper is defined by
\begin{equation}
^{\text{CAM}}\mathbf{T}_{\text{ECM}} = \begin{bmatrix}
^{\text{CAM}}\mathbf{R}_{\text{ECM}} & \vec{t} \\
\vec{0}T  &1
\end{bmatrix} =
\begin{bmatrix}
r_{11} & r_{12} & r_{13} & t_1(\vec{x}) \\
r_{21} & r_{22} & r_{23} & t_2(\vec{x}) \\
r_{31} & r_{32} & r_{33} & t_3(\vec{x}) \\
0 & 0 & 0 & 1
\end{bmatrix}
\text{CAM}
\text{ECM}
\end{equation}
where each individual parameter $(t_1, t_2, t_3)$ describing the translation component of the transformation and the remaining $r_{ij}$ are the conversion result from the 6D rotation formula. Each translation component is a continuous scalar value and is directly the output of the network, therefore they are differentiable.

For the rotation matrix, the Gram-Schmidt orthogonalisation is used to convert the 6D rotation to the orthogonal matrix. Given the output of the network for the rotation are the two vectors $\vec{u} = [u_1(\vec{x}), u_2(\vec{x}), u_3(\vec{x})]^T$ and $\vec{v} = [v_1(\vec{x}), v_2(\vec{x}), v_3(\vec{x})]^T$, the rotation can be written as follows.
\begin{eqnarray}
\begin{split}
\vec{r}_x &= \frac{\vec{u}_1}{||\vec{u}_1||} \\
\vec{r}_y &= \frac{\vec{v} - (\vec{u}^T\vec{v})\vec{u}}{||\vec{v} - (\vec{u}^T\vec{v})\vec{u}||} \\
\vec{r}_z &= \vec{u}\times\vec{v} \\
^{\text{CAM}}\mathbf{R}_{\text{ECM}} &= \begin{bmatrix}
\vec{r}_x & \vec{r}_y & \vec{r}_z 
\end{bmatrix} 
&= \begin{bmatrix}
r_{11} & r_{12} & r_{13} \\
r_{21} & r_{22} & r_{23} \\
r_{31} & r_{32} & r_{33} 
\end{bmatrix}
\end{split}
\label{eq:R-r3} 
\end{eqnarray} 
As can be seen from the equations above that, all of the operations can be differentiated, therefore the gradient of the conversion from the network output to the hand-eye equation is valid. Similarly, the term $\mathfrak{L}_{\text{rcm}}$ is also differentiable as well, as it only contains the norm function and arc-cosine function which are both differentiable.
\subsection*{Re-projection loss}
\begin{equation}
\mathfrak{L}_{\text{proj}} = \sum_{j=1}^2\sum_{i = 1}^N w_j\lvert\lvert\mathbf{p}_{1, j} - f(^{\text{CAM}}\mathbf{T}_{\text{PSM}j})\rvert\rvert
\label{eq:reproj}
\end{equation}
The re-projection function uses intrinsic and distortion parameters to transform the position and the orientation to the camera frame and it has been used in neural network appliction before in \cite{calibRCNN}. Once taken the derivative, the only term in the chain rule that is a function of $\vec{x}$ is $^{\text{CAM}}\mathbf{T}_{\text{PSM}j}$ which can be broken down to $^{\text{CAM}}\mathbf{T}_{\text{ECM}}(\vec{x})\ ^{\text{ECM}}\mathbf{T}_{\text{PSM}j}$ and it is previously shown that the gradient of this term exists.
\subsection*{Differentiation of re-projection}
\begin{eqnarray}
\begin{split}
\mathfrak{L}_{\text{diff}} &= \sum_{j=1}^2\sum_{i = 1}^N w_j\lvert\lvert\dot{\mathbf{p}}_{1, i} - \dot{f}(^{\text{CAM}}\mathbf{T}_{\text{PSM}j})\frac{\partial ^{\text{CAM}}\mathbf{T}_{\text{PSM}j}}{\partial t}\rvert\rvert \\
\text{where}\quad\frac{\partial ^{\text{CAM}}\mathbf{T}_{\text{PSM}j}}{\partial t} &= ^{\text{CAM}}\dot{\mathbf{T}}_{\text{ECM}}\ ^{\text{ECM}}\mathbf{T}_{\text{PSM}j} + \ ^{\text{CAM}}\mathbf{T}_{\text{ECM}}\ ^{\text{ECM}}\dot{\mathbf{T}}_{\text{PSM}j}
\label{eq:reproj-diff}
\end{split}
\end{eqnarray}

\bibliography{myBib}

\end{document}
